# Supplementary material for: Violence Detection in Videos
Source: arXiv:2109.08941 source file (2021-09-18)
Supplement: Supplementary file 1 [file AppendixA.tex]

% Appendix A

\chapter{Appendix Title Here} % Main appendix title

\label{AppendixA} % For referencing this appendix elsewhere, use \ref{AppendixA}

\lhead{Appendix A. \emph{Appendix Title Here}} % This is for the header on each page - perhaps a shortened title

Write your Appendix content here.
